# Supplementary material for: Contributing Components of Metabolic Energy Models to Metabolic Cost Estimations in Gait
Source: arXiv:2310.12083 source file (2023-10-18)
Supplement: Supplementary file 1 [file 09X_Appendix.tex]

\begin{tabular}{llrr}
\toprule
  name &              vars &     rmse &      rmc \\
\midrule
muscle &       [0 1 2 3 6] & 0.862034 & 0.937788 \\
 joint &           [0 2 3] & 0.862162 & 0.935519 \\
muscle &       [1 4 5 6 7] & 0.898562 & 0.921129 \\
muscle &     [0 1 2 3 5 6] & 0.901412 & 0.932690 \\
muscle &         [1 4 5 6] & 0.909401 & 0.914650 \\
muscle &         [1 3 5 6] & 0.916114 & 0.925316 \\
muscle &       [0 1 2 3 4] & 0.936444 & 0.915985 \\
 joint &           [0 1 2] & 0.941836 & 0.925861 \\
muscle &           [1 4 6] & 0.942412 & 0.907117 \\
muscle &           [0 1 2] & 0.950875 & 0.934536 \\
muscle &       [0 2 4 5 6] & 0.959018 & 0.899773 \\
muscle &       [0 2 5 6 7] & 0.975108 & 0.903441 \\
muscle &       [0 1 2 3 5] & 0.982091 & 0.932419 \\
muscle &       [1 3 4 5 6] & 0.988606 & 0.907822 \\
muscle &           [0 2 3] & 0.992261 & 0.928660 \\
muscle &         [0 1 4 6] & 0.994101 & 0.917506 \\
muscle &         [1 3 6 7] & 1.001596 & 0.939072 \\
muscle &           [1 2 6] & 1.012853 & 0.901061 \\
muscle &           [1 2 3] & 1.019131 & 0.911125 \\
muscle &         [0 2 3 4] & 1.020241 & 0.882069 \\
muscle &         [1 2 4 6] & 1.027601 & 0.908115 \\
muscle &   [0 1 2 3 5 6 7] & 1.028363 & 0.904380 \\
muscle & [0 1 2 3 4 5 6 7] & 1.028872 & 0.902788 \\
muscle &         [1 2 3 7] & 1.030756 & 0.876729 \\
muscle &       [1 2 4 5 7] & 1.031255 & 0.881287 \\
muscle &     [0 1 2 4 5 6] & 1.031975 & 0.908415 \\
 joint &           [1 2 3] & 1.035554 & 0.902080 \\
muscle &             [0 6] & 1.038161 & 0.902738 \\
muscle &     [1 3 4 5 6 7] & 1.042934 & 0.901790 \\
 joint &         [0 1 2 3] & 1.045675 & 0.919109 \\
muscle &         [1 2 4 7] & 1.053349 & 0.898934 \\
muscle &       [0 1 2 5 7] & 1.054521 & 0.903710 \\
muscle &     [1 2 4 5 6 7] & 1.055144 & 0.916830 \\
muscle &     [0 1 2 3 4 7] & 1.056182 & 0.909757 \\
muscle &     [0 1 3 4 5 6] & 1.058072 & 0.886507 \\
muscle &     [1 2 3 4 6 7] & 1.059048 & 0.907117 \\
 joint &             [0 1] & 1.060835 & 0.910754 \\
muscle &       [1 2 4 5 6] & 1.062641 & 0.872436 \\
muscle &       [1 2 3 4 6] & 1.063289 & 0.883630 \\
muscle &     [0 1 2 4 5 7] & 1.063568 & 0.909100 \\
muscle &       [0 1 2 4 5] & 1.064125 & 0.914712 \\
muscle &     [0 1 2 4 6 7] & 1.067836 & 0.901294 \\
muscle &       [1 2 3 6 7] & 1.068978 & 0.892834 \\
muscle &         [1 2 5 6] & 1.069869 & 0.886017 \\
muscle &     [2 3 4 5 6 7] & 1.075483 & 0.927912 \\
muscle &         [0 2 3 6] & 1.081391 & 0.910165 \\
muscle &         [1 2 4 5] & 1.081568 & 0.873749 \\
muscle &     [0 1 3 4 6 7] & 1.084416 & 0.876762 \\
muscle &       [1 2 3 5 6] & 1.088208 & 0.871242 \\
muscle &       [1 3 5 6 7] & 1.088867 & 0.906433 \\
muscle &         [0 1 2 4] & 1.090272 & 0.864834 \\
muscle &       [0 1 3 4 6] & 1.091040 & 0.869589 \\
muscle &             [1 2] & 1.092070 & 0.862009 \\
muscle &           [1 2 5] & 1.093404 & 0.853089 \\
muscle &         [1 2 3 4] & 1.098009 & 0.857614 \\
muscle &       [0 1 2 6 7] & 1.099652 & 0.909811 \\
muscle &           [1 6 7] & 1.100682 & 0.905177 \\
muscle &         [0 3 6 7] & 1.100690 & 0.906208 \\
muscle &       [0 1 2 4 6] & 1.100960 & 0.910263 \\
muscle &     [0 1 3 5 6 7] & 1.103568 & 0.903946 \\
muscle &     [0 1 2 3 6 7] & 1.104824 & 0.857961 \\
muscle &           [1 2 4] & 1.114515 & 0.859537 \\
muscle &       [1 2 3 5 7] & 1.114599 & 0.870185 \\
muscle &       [0 2 3 4 7] & 1.121199 & 0.868785 \\
muscle &     [1 2 3 5 6 7] & 1.121280 & 0.913708 \\
muscle &     [0 1 2 3 5 7] & 1.122381 & 0.869542 \\
muscle &         [0 2 4 7] & 1.123724 & 0.901760 \\
muscle &         [0 3 5 6] & 1.128799 & 0.891086 \\
muscle &           [0 2 7] & 1.132060 & 0.860798 \\
muscle &       [1 2 4 6 7] & 1.132321 & 0.889803 \\
muscle &         [1 2 3 6] & 1.135664 & 0.862831 \\
muscle &         [2 3 4 7] & 1.136192 & 0.897303 \\
muscle &         [4 5 6 7] & 1.136706 & 0.910844 \\
muscle &       [0 2 3 6 7] & 1.139038 & 0.914412 \\
muscle &         [0 2 5 6] & 1.142239 & 0.878788 \\
muscle &           [0 2 5] & 1.143430 & 0.856922 \\
muscle &       [1 2 5 6 7] & 1.144098 & 0.898000 \\
 joint &             [0 2] & 1.146851 & 0.918728 \\
muscle &           [0 1 6] & 1.148236 & 0.824802 \\
muscle &     [0 2 4 5 6 7] & 1.148801 & 0.883643 \\
muscle &           [4 5 6] & 1.149404 & 0.869579 \\
muscle &         [1 5 6 7] & 1.149438 & 0.871177 \\
muscle &         [2 4 5 6] & 1.149917 & 0.883724 \\
muscle &     [0 1 4 5 6 7] & 1.153097 & 0.890883 \\
muscle &         [1 2 5 7] & 1.153319 & 0.779413 \\
muscle &           [0 4 5] & 1.153881 & 0.811806 \\
muscle &     [0 2 3 4 5 7] & 1.154411 & 0.846085 \\
muscle &           [0 5 6] & 1.154809 & 0.899059 \\
muscle &         [3 5 6 7] & 1.155624 & 0.907129 \\
muscle &   [0 2 3 4 5 6 7] & 1.156222 & 0.888457 \\
muscle &   [1 2 3 4 5 6 7] & 1.157346 & 0.838114 \\
muscle &       [0 2 4 6 7] & 1.158451 & 0.868295 \\
muscle &         [1 2 3 5] & 1.159442 & 0.878078 \\
muscle &   [0 1 2 3 4 6 7] & 1.159556 & 0.861387 \\
muscle &       [0 1 3 6 7] & 1.160729 & 0.867336 \\
muscle &           [0 2 4] & 1.160918 & 0.860404 \\
muscle &     [0 1 2 3 4 6] & 1.163467 & 0.833027 \\
muscle &       [2 3 4 5 6] & 1.166304 & 0.852076 \\
muscle &         [1 4 6 7] & 1.168634 & 0.858665 \\
muscle &         [0 1 2 5] & 1.169366 & 0.862811 \\
muscle &       [2 4 5 6 7] & 1.171016 & 0.872886 \\
muscle &     [0 2 3 4 5 6] & 1.174621 & 0.882570 \\
muscle &         [0 1 5 6] & 1.178187 & 0.812193 \\
muscle &         [0 2 4 6] & 1.178875 & 0.891340 \\
muscle &         [0 2 3 5] & 1.179845 & 0.780623 \\
muscle &         [1 2 6 7] & 1.180795 & 0.852799 \\
muscle &           [2 3 7] & 1.181664 & 0.891355 \\
muscle &         [0 1 2 6] & 1.182212 & 0.859439 \\
muscle &         [0 1 3 4] & 1.183604 & 0.830838 \\
muscle &         [0 2 6 7] & 1.184355 & 0.892522 \\
muscle &         [0 4 5 6] & 1.189183 & 0.818892 \\
muscle &         [0 2 5 7] & 1.189880 & 0.835945 \\
muscle &           [2 5 7] & 1.191718 & 0.915809 \\
muscle &     [0 3 4 5 6 7] & 1.192748 & 0.862904 \\
muscle &       [3 4 5 6 7] & 1.194244 & 0.919865 \\
muscle &         [0 2 3 7] & 1.195991 & 0.862801 \\
muscle &       [2 3 4 6 7] & 1.199970 & 0.905759 \\
muscle &         [3 4 5 6] & 1.200355 & 0.884139 \\
muscle &       [0 1 4 6 7] & 1.201765 & 0.854657 \\
 joint &             [2 3] & 1.202300 & 0.860450 \\
muscle &   [0 1 2 3 4 5 6] & 1.208916 & 0.815251 \\
muscle &     [0 1 2 3 4 5] & 1.213080 & 0.789271 \\
muscle &         [2 3 5 6] & 1.214146 & 0.890100 \\
muscle &       [2 3 5 6 7] & 1.214946 & 0.903796 \\
 joint &           [0 1 3] & 1.216011 & 0.894292 \\
muscle &     [0 2 3 5 6 7] & 1.221089 & 0.868350 \\
muscle &   [0 1 2 4 5 6 7] & 1.223820 & 0.896137 \\
muscle &         [2 4 5 7] & 1.224031 & 0.828969 \\
muscle &         [1 3 4 6] & 1.224109 & 0.846090 \\
muscle &           [2 3 5] & 1.224438 & 0.848930 \\
muscle &             [2 7] & 1.226508 & 0.854414 \\
muscle &         [2 3 6 7] & 1.227116 & 0.892875 \\
muscle &         [2 3 4 5] & 1.227167 & 0.856143 \\
muscle &       [1 2 3 4 5] & 1.229461 & 0.798823 \\
muscle &       [0 2 3 5 6] & 1.230643 & 0.830168 \\
muscle &           [0 2 6] & 1.230664 & 0.832390 \\
muscle &       [0 3 5 6 7] & 1.230693 & 0.809552 \\
muscle &           [2 3 4] & 1.231240 & 0.850085 \\
muscle &           [2 4 6] & 1.234249 & 0.853345 \\
muscle &       [0 4 5 6 7] & 1.238287 & 0.852523 \\
muscle &     [0 1 2 5 6 7] & 1.238291 & 0.865848 \\
muscle &         [0 1 3 6] & 1.239289 & 0.813417 \\
muscle &       [0 1 3 5 6] & 1.239933 & 0.782630 \\
muscle &         [2 4 6 7] & 1.241233 & 0.887087 \\
muscle &       [0 1 5 6 7] & 1.242691 & 0.739362 \\
muscle &   [0 1 2 3 4 5 7] & 1.242826 & 0.834235 \\
muscle &       [0 2 3 4 6] & 1.243407 & 0.854291 \\
muscle &         [0 1 6 7] & 1.243625 & 0.779552 \\
 joint &               [1] & 1.244927 & 0.838506 \\
muscle &       [0 2 3 5 7] & 1.247666 & 0.738275 \\
muscle &           [1 2 7] & 1.249999 & 0.811661 \\
muscle &           [2 4 7] & 1.250886 & 0.859791 \\
muscle &           [3 5 6] & 1.252528 & 0.875034 \\
muscle &           [2 3 6] & 1.253799 & 0.861012 \\
muscle &             [2 5] & 1.256129 & 0.863267 \\
muscle &           [1 5 6] & 1.259035 & 0.784538 \\
muscle &         [0 5 6 7] & 1.260187 & 0.794063 \\
muscle &       [0 1 3 4 5] & 1.261423 & 0.807991 \\
muscle &             [2 4] & 1.262770 & 0.809267 \\
muscle &         [2 5 6 7] & 1.273375 & 0.900042 \\
muscle &       [0 2 3 4 5] & 1.274223 & 0.800415 \\
muscle &         [2 3 5 7] & 1.275804 & 0.862418 \\
muscle &     [1 2 3 4 5 7] & 1.277583 & 0.806112 \\
muscle &         [0 4 6 7] & 1.279482 & 0.772105 \\
muscle &   [0 1 3 4 5 6 7] & 1.280174 & 0.791905 \\
muscle &               [0] & 1.283217 & 0.751746 \\
muscle &             [0 2] & 1.285847 & 0.825775 \\
muscle &         [0 1 4 5] & 1.286636 & 0.775491 \\
muscle &       [2 3 4 5 7] & 1.288554 & 0.822706 \\
muscle &       [0 1 3 5 7] & 1.291068 & 0.730579 \\
muscle &         [0 2 4 5] & 1.295625 & 0.798388 \\
muscle &       [1 3 4 6 7] & 1.299329 & 0.828548 \\
muscle &         [0 1 4 7] & 1.300746 & 0.779642 \\
muscle &           [3 6 7] & 1.304171 & 0.796309 \\
muscle &       [0 1 3 4 7] & 1.314443 & 0.685414 \\
muscle &         [2 3 4 6] & 1.314769 & 0.786233 \\
muscle &           [1 3 6] & 1.314986 & 0.822868 \\
muscle &       [1 2 3 4 7] & 1.317509 & 0.778129 \\
muscle &           [2 6 7] & 1.317954 & 0.736782 \\
muscle &       [0 3 4 6 7] & 1.323000 & 0.749028 \\
muscle &         [0 1 2 7] & 1.323711 & 0.810993 \\
muscle &         [0 3 4 7] & 1.326675 & 0.753751 \\
muscle &           [0 3 6] & 1.329316 & 0.755855 \\
muscle &         [0 1 3 5] & 1.329608 & 0.643541 \\
muscle &           [2 4 5] & 1.341666 & 0.811994 \\
muscle &       [0 1 4 5 7] & 1.351951 & 0.760170 \\
muscle &       [0 3 4 5 6] & 1.358428 & 0.803119 \\
muscle &           [2 5 6] & 1.358827 & 0.782476 \\
muscle &             [4 6] & 1.362966 & 0.831746 \\
muscle &           [1 4 5] & 1.366685 & 0.675451 \\
muscle &           [0 1 3] & 1.373604 & 0.648284 \\
muscle &           [0 4 7] & 1.377038 & 0.697210 \\
 joint &             [1 2] & 1.380553 & 0.801107 \\
muscle &       [0 1 4 5 6] & 1.389963 & 0.715410 \\
muscle &             [2 6] & 1.390952 & 0.793646 \\
muscle &       [1 3 4 5 7] & 1.394171 & 0.686050 \\
 joint &             [1 3] & 1.395355 & 0.856225 \\
muscle &         [0 3 4 5] & 1.397235 & 0.655901 \\
muscle &             [3 6] & 1.398997 & 0.827969 \\
muscle &           [5 6 7] & 1.402666 & 0.752453 \\
muscle &           [0 5 7] & 1.404766 & 0.719560 \\
muscle &     [1 2 3 4 5 6] & 1.417373 & 0.669159 \\
muscle &           [0 1 5] & 1.418894 & 0.623509 \\
muscle &       [0 1 2 3 7] & 1.426906 & 0.768319 \\
muscle &       [0 2 4 5 7] & 1.429510 & 0.617453 \\
muscle &             [0 1] & 1.437468 & 0.632953 \\
muscle &           [4 6 7] & 1.460513 & 0.565046 \\
muscle &           [0 6 7] & 1.462758 & 0.761254 \\
muscle &         [1 3 5 7] & 1.464801 & 0.668230 \\
muscle &           [0 3 4] & 1.466186 & 0.609746 \\
muscle &             [0 4] & 1.466571 & 0.721340 \\
muscle &           [1 3 4] & 1.474199 & 0.661827 \\
muscle &         [0 1 5 7] & 1.475424 & 0.656282 \\
muscle &         [0 1 2 3] & 1.484116 & 0.648841 \\
muscle &             [6 7] & 1.490020 & 0.759879 \\
muscle &       [0 1 2 5 6] & 1.493769 & 0.699999 \\
 joint &               [2] & 1.500217 & 0.685472 \\
muscle &             [1 7] & 1.502623 & 0.579680 \\
muscle &         [0 4 5 7] & 1.507359 & 0.654516 \\
muscle &     [0 1 3 4 5 7] & 1.509389 & 0.491774 \\
muscle &           [0 1 4] & 1.514866 & 0.475338 \\
muscle &           [0 4 6] & 1.520192 & 0.669569 \\
muscle &         [3 4 6 7] & 1.526608 & 0.721263 \\
muscle &               [2] & 1.530742 & 0.536733 \\
muscle &           [3 4 6] & 1.548983 & 0.426343 \\
muscle &         [0 3 4 6] & 1.550555 & 0.662722 \\
 joint &             [0 3] & 1.552482 & 0.797129 \\
muscle &             [5 6] & 1.561531 & 0.601651 \\
muscle &             [0 5] & 1.564198 & 0.567122 \\
muscle &             [0 3] & 1.572320 & 0.508614 \\
muscle &         [1 3 4 7] & 1.573034 & 0.411041 \\
muscle &           [0 3 5] & 1.582912 & 0.501081 \\
muscle &             [1 6] & 1.588637 & 0.669553 \\
muscle &           [0 1 7] & 1.607467 & 0.592952 \\
muscle &             [2 3] & 1.620747 & 0.534932 \\
muscle &         [0 1 3 7] & 1.634526 & 0.339357 \\
muscle &     [0 2 3 4 6 7] & 1.641039 & 0.541720 \\
muscle &           [1 4 7] & 1.661429 & 0.244150 \\
muscle &               [6] & 1.664395 & 0.363137 \\
muscle &         [0 3 5 7] & 1.680632 & 0.264138 \\
muscle &             [3 5] & 1.685445 & 0.244049 \\
muscle &           [1 3 5] & 1.685731 & 0.244959 \\
muscle &         [1 3 4 5] & 1.695259 & 0.248901 \\
muscle &           [0 3 7] & 1.698096 & 0.466205 \\
muscle &             [5 7] & 1.706285 & 0.249734 \\
muscle &       [0 1 2 4 7] & 1.721356 & 0.243989 \\
muscle &             [1 5] & 1.727026 & 0.224811 \\
muscle &               [3] & 1.729736 & 0.206061 \\
muscle &           [3 4 5] & 1.744850 & 0.230118 \\
muscle &               [5] & 1.746961 & 0.212708 \\
muscle &           [3 5 7] & 1.758480 & 0.207128 \\
muscle &           [3 4 7] & 1.767675 & 0.231904 \\
muscle &         [3 4 5 7] & 1.769937 & 0.217222 \\
muscle &             [1 3] & 1.792956 & 0.225857 \\
muscle &             [4 7] & 1.795842 & 0.220064 \\
muscle &           [1 3 7] & 1.796493 & 0.316441 \\
 joint &               [0] & 1.816211 & 0.637204 \\
muscle &           [1 5 7] & 1.837476 & 0.203184 \\
muscle &             [1 4] & 1.839489 & 0.213883 \\
muscle &             [0 7] & 1.849930 & 0.417697 \\
muscle &             [4 5] & 1.850354 & 0.201260 \\
muscle &             [3 4] & 1.857152 & 0.218488 \\
muscle &       [0 3 4 5 7] & 1.862312 & 0.412640 \\
 joint &               [3] & 1.866445 & 0.395003 \\
muscle &               [7] & 1.866844 & 0.181870 \\
muscle &         [1 4 5 7] & 1.870141 & 0.188074 \\
muscle &               [4] & 1.873145 & 0.189752 \\
muscle &             [3 7] & 1.904058 & 0.195023 \\
muscle &               [1] & 1.914270 & 0.174663 \\
muscle &           [4 5 7] & 2.025062 & 0.160755 \\
\bottomrule
\end{tabular}
